# Supplementary material for: Controlling the Interaction of Electron and Nuclear Spins in a Tunnel-Coupled Quantum Dot
Source: arXiv:1010.3330 source file (2011-02-01)
Supplement: Supplementary file 1 [file supplement.pdf]

# Supplementary Information to “Controlling the Interaction of Electron and Nuclear Spins in a Tunnel-Coupled Quantum Dot”

C. Kloeffer,<sup>1</sup> P. A. Dalgarno,<sup>2</sup> B. Urbaszek,<sup>3</sup> B. D. Gerardot,<sup>2</sup> D. Brunner,<sup>2</sup> P. M. Petroff,<sup>4</sup> D. Loss,<sup>1</sup> and R. J. Warburton<sup>1,2</sup>

<sup>1</sup>*Department of Physics, University of Basel, Klingelbergstrasse 82, CH-4056 Basel, Switzerland*

<sup>2</sup>*School of Engineering and Physical Sciences, Heriot-Watt University, Edinburgh EH14 4AS, UK*

<sup>3</sup>*Université de Toulouse, INSA-CNRS-UPS, LPCNO, 135 Avenue de Rangueil, 31077 Toulouse, France*

<sup>4</sup>*Materials Department, University of California, Santa Barbara, California 93106, USA*

(Dated: February 1, 2011)

In “Controlling the Interaction of Electron and Nuclear Spins in a Tunnel-Coupled Quantum Dot” [1] we report a technique for manipulating the nuclear spins and the emission polarization from a single optically active quantum dot. In order to describe this system theoretically, we divide the calculation into two interlinked parts. Process I: the laser field induces dynamics in a five-level electronic system. The final event is  $X^{1-}$  recombination. Process II: nuclear spin polarization builds up via electron-nuclear spin flip-flop processes. Process I provides an unpaired electron spin as input to process II. Conversely, process II creates an Overhauser field which is an input to process I. In the presence of nuclear spin leakage, a master equation for the nuclear spin polarization  $\langle I_z \rangle$  has stable solutions where  $d\langle I_z \rangle/dt = 0$ . Associated with the stable solutions for  $\langle I_z \rangle$  are particular values of the Overhauser field, and hence particular values of the photoluminescence energies and intensities for the two light polarizations,  $\sigma^+$  and  $\sigma^-$ . The details of this calculation are described here along with the input parameters. The results of the calculation can be compared directly with the experimental results (Fig. 2 of [1]). Furthermore, we comment on the consequences of the theory for the fluctuations of the nuclear spin ensemble.

## I. COHERENT EVOLUTION OF THE FIVE-LEVEL SYSTEM

The dynamics of the five-level quantum system induced by the laser field are calculated with the density matrix. The ground state is the empty dot,  $|0\rangle$ . There are two neutral exciton states,  $|\uparrow\downarrow\rangle$  (hole spin up, electron spin down) and  $|\downarrow\uparrow\rangle$  (hole spin down, electron spin up). Defining the ground state energy as zero, the diagonal terms of the Hamiltonian matrix  $\hat{H}$  are

$$\begin{aligned}\langle\uparrow\downarrow|\hat{H}|\uparrow\downarrow\rangle &= \hbar\omega_0 + 1/2 \cdot (g_X\mu_B B_z - A\langle I_z \rangle), \\ \langle\downarrow\uparrow|\hat{H}|\downarrow\uparrow\rangle &= \hbar\omega_0 - 1/2 \cdot (g_X\mu_B B_z - A\langle I_z \rangle),\end{aligned}$$

where  $\hbar\omega_0$  is the eigenenergy of  $|\uparrow\downarrow\rangle$  and  $|\downarrow\uparrow\rangle$  in the absence of a magnetic field. Coupling to the external magnetic field  $B_z$  is determined by the exciton g-factor  $g_X$ . The electron also interacts with the internal (Overhauser) magnetic field, given by the expectation value of the nuclear spin  $\vec{z}$  projection  $\langle I_z \rangle$  (in units of  $\hbar$ ) and the averaged effective coupling constant  $A$ . The  $\sigma^+$ -polarized laser of angular frequency  $\omega = \omega_0 + \delta$ , with  $\hbar\delta$  as detuning, drives the  $|0\rangle \leftrightarrow |\uparrow\downarrow\rangle$  but not the  $|0\rangle \leftrightarrow |\downarrow\uparrow\rangle$  transition on account of the selection rules. As the laser is always close to the resonance, the rotating wave approximation applies. The off-diagonal elements in the Hamiltonian are

$$\begin{aligned}\langle 0|\hat{H}|\uparrow\downarrow\rangle &= \hbar\Omega/2 \cdot e^{i\omega t}, \\ \langle\downarrow\uparrow|\hat{H}|\uparrow\downarrow\rangle &= \hbar\omega_{fs}/2,\end{aligned}$$

where  $\hbar\Omega$  is the optical Rabi energy, and  $\hbar\omega_{fs}$  is the fine structure splitting arising from the anisotropic part of the electron-hole exchange [2]. The two exciton states can decay either by spontaneous emission to the ground state at rate  $\tau_0^{-1}$ , or by tunneling of an electron into the quantum dot at rate  $\tau_{in}^{-1}$ . Tunneling converts  $|\uparrow\downarrow\rangle$  into the  $X^{1-}$  state  $|\uparrow\downarrow\uparrow\rangle$ ;  $|\downarrow\uparrow\rangle$  into the other  $X^{1-}$  state  $|\downarrow\uparrow\downarrow\rangle$ . The trion states decay by spontaneous recombination, at rate  $\tau_1^{-1}$ , to states  $|\uparrow\rangle$ ,  $|\downarrow\rangle$ , respectively. Figure 4 (top) of [1] summarizes all the coherent couplings and decay processes.

At  $t = 0$ , the entire population resides in the ground state. The probability of finding the system in state  $|s\rangle$  at times  $t > 0$  corresponds to element  $\langle s|\hat{\rho}|s\rangle$  of the density matrix  $\hat{\rho}$ , and we use the master equation with the decay processes in the Lindblad form,

$$\begin{aligned}\frac{d}{dt}\hat{\rho} &= -\frac{i}{\hbar} [\hat{H}, \hat{\rho}] + D\hat{\rho}, \\ D\hat{\rho} &= \sum_{m,n} \Gamma_{|m\rangle \rightarrow |n\rangle} \left( |n\rangle \langle m| \hat{\rho} |m\rangle \langle n| - \frac{1}{2} |m\rangle \langle m| \hat{\rho} - \frac{1}{2} \hat{\rho} |m\rangle \langle m| \right),\end{aligned}$$

to calculate its coherent evolution [3]. The dissipator  $D\hat{\rho}$  accounts for the decay processes, where  $\Gamma_{|m\rangle \rightarrow |n\rangle}$  is the transition rate from state  $|m\rangle$  to  $|n\rangle$ .

Of particular interest are the trion populations,  $p_{|\uparrow\downarrow\uparrow\rangle} \equiv \langle \uparrow\downarrow\uparrow | \hat{\rho} | \uparrow\downarrow\uparrow \rangle$ ,  $p_{|\downarrow\uparrow\downarrow\rangle} \equiv \langle \downarrow\uparrow\downarrow | \hat{\rho} | \downarrow\uparrow\downarrow \rangle$ , since they determine both the  $X^{1-}$  emission intensity and the probability of creating a conduction level electron with spin up (down) after trion recombination. The spontaneous  $X^{1-}$  recombination time is  $\tau_1$ , and we hence take  $(p_{|\uparrow\downarrow\uparrow\rangle}/\tau_1)|_{t=\tau_1}$  and  $(p_{|\downarrow\uparrow\downarrow\rangle}/\tau_1)|_{t=\tau_1}$  as the rates of creating an  $\uparrow$ ,  $\downarrow$  electron, respectively. This approximation, essentially that the dynamics approach the steady state faster than spontaneous recombination, is well justified for laser energies near resonance. For large detunings, the approximation works less well, but going beyond this approximation would greatly complicate the calculation at the expense of transparency. Figure 1 (left) shows the evolution of the trion population as calculated in the five-level system for a laser energy in the region of the bistability. The parameters are the same as used in the main article [1], summarized in detail in section V below. For positive (negative) nuclear spin polarization, the  $|\uparrow\downarrow\uparrow\rangle$  ( $|\downarrow\uparrow\downarrow\rangle$ ) state is preferentially occupied, leading to  $\sigma^+$  ( $\sigma^-$ ) emission and dynamic nuclear spin polarization in positive (negative)  $\hat{z}$  direction.

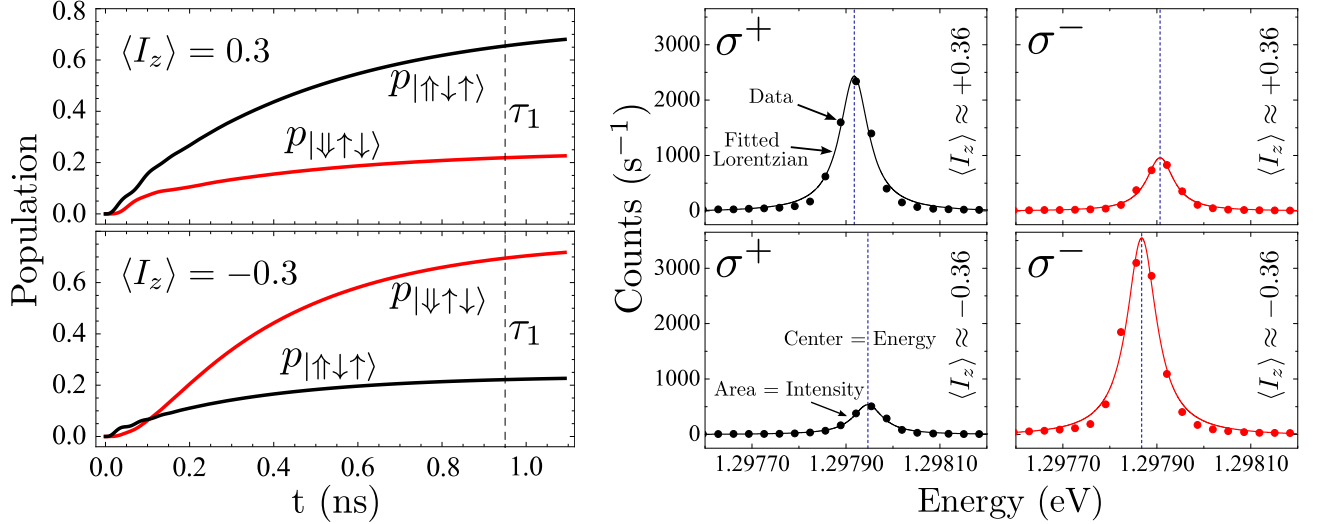

FIG. 1. Left: Simulation of the trion occupation probabilities  $p_{|\uparrow\downarrow\uparrow\rangle}$  and  $p_{|\downarrow\uparrow\downarrow\rangle}$  in the five-level system of ground state, neutral and negatively charged excitons, taking the entire population in the ground state at time  $t = 0$ . The parameters are the same as used in the main article [1], summarized in detail in section V, with the detuning  $\hbar\delta$  fixed in the region of bistability. Depending on the value of  $\langle I_z \rangle$ , either  $|\uparrow\downarrow\uparrow\rangle$  or  $|\downarrow\uparrow\downarrow\rangle$  is preferentially occupied after the  $X^{1-}$  recombination time  $\tau_1$ , determining the rate of creating an  $\uparrow$ ,  $\downarrow$  electron via optical recombination. Right: Measured counts-energy spectra with the laser tuned to the region of bistability. The dot, at 4.2 K, is the same as in Figs. 1-3 of [1] and the energy of the detected signal corresponds to  $X^{1-}$ . The experimental data are fitted to Lorentzians, yielding both the energies  $E(\sigma^{+/-})$  (center of curve) and the signal intensities  $S(\sigma^{+/-})$  (area under curve). A clear shift in the energies is observed, arising from different nuclear spin polarizations  $\langle I_z \rangle$ . As expected from the theory (left), the  $\sigma^+$  signal is pronounced when the nuclear spin polarization is positive, and vice versa. Both theory and experiment use a  $\sigma^+$  pump and an external field of  $B_z = +0.5$  T.

## II. FLIP-FLOP OF ELECTRON AND NUCLEAR SPIN

At time  $t = \tau_1$ , after  $X^{1-}$  recombination, the quantum dot is in the  $|e\rangle$  state and contains a free electron. This electron interacts with the  $N$  nuclear spins in the quantum dot before it tunnels into the Fermi sea at rate  $\tau_{\text{out}}^{-1}$ . Since the conduction level electron has an s-type Bloch function, its coupling to the nuclear spins is well described by the contact hyperfine interaction with effective Hamiltonian

$$\hat{H}_{\text{hf}} = \nu_0 \sum_k A_k^j |\psi(\vec{R}_k)|^2 \vec{I}_k \cdot \vec{S}.$$

Here  $A^j$  are the effective hyperfine coupling constants for atoms of type  $j$ ,  $\nu_0$  denotes the volume per atom,  $\psi(\vec{R}_k)$  is the electron wave function at nucleus  $k$ , and  $\vec{I}$ ,  $\vec{S}$  are the nuclear and electron spins in units of  $\hbar$  [4]. We assume homogeneous coupling, which yields

$$\hat{H}_{\text{hf}} \simeq \frac{A}{N} \sum_k \vec{I}_k \cdot \vec{S} \equiv A \langle \vec{I} \rangle \cdot \vec{S}, \quad (1)$$

a result used in the diagonal elements of the five-level system. Based on  $\text{In}_{0.5}\text{Ga}_{0.5}\text{As}$ , we take  $A \approx 90 \mu\text{eV}$  as the averaged effective coupling constant [4] and  $I = 0.75 \cdot 3/2 + 0.25 \cdot 9/2 = 2.25$  as averaged nuclear spin quantum number. Adding the

Zeeman term  $\hat{H}_{\text{ext}}$ , with  $g_e$  as electron g-factor, the total Hamiltonian reads

$$\hat{H}_{\text{ext}} + \hat{H}_{\text{hf}} = g_e \mu_B B_z S_z + A \langle I_z \rangle S_z + \frac{A}{2N} \sum_k (I_k^+ S^- + I_k^- S^+), \quad (2)$$

where  $I_k^\pm \equiv I_k^x \pm i I_k^y$  and  $S^\pm \equiv S_x \pm i S_y$  are ladder operators, such that the final term describes a flip-flop of electron and nuclear spin. In the following it is assumed that the electron has spin up; the calculation for spin down is analogous.

To estimate the flip-flop probability as a function of net nuclear polarization, we calculate the time evolution in the effective 2D system  $\{|M, \uparrow\rangle, |M+1, \downarrow\rangle\}$ , where  $|M\rangle$  represents the ensemble of nuclear spin states with  $\bar{z}$  projection  $M = N \langle I_z \rangle$ . With the system in state  $|M, \uparrow\rangle$  at time  $t' \equiv t - \tau_1 = 0$ , one finds from the von Neumann equation [3] that the population of  $|M+1, \downarrow\rangle$  oscillates in time according to

$$p_{|M+1, \downarrow\rangle} = \frac{4\gamma}{4\gamma + \xi} \sin^2 \left( \frac{\sqrt{4\gamma + \xi}}{2\hbar} t' \right), \quad (3)$$

where

$$\gamma \equiv \left| \langle M+1, \downarrow | \hat{H}_{\text{hf}} | M, \uparrow \rangle \right|^2, \\ \xi \equiv \left| \langle M+1, \downarrow | \hat{H}_{\text{ext}} + \hat{H}_{\text{hf}} | M+1, \downarrow \rangle - \langle M, \uparrow | \hat{H}_{\text{ext}} + \hat{H}_{\text{hf}} | M, \uparrow \rangle \right|^2.$$

From Eq. (2),  $\xi = (g_e \mu_B B_z + A \langle I_z \rangle)^2$ . Simple results for  $\gamma$  only exist when the nuclear spins are either fully correlated or fully uncorrelated, neither of which is the case here. With  $\gamma = \frac{A^2}{4N} (I - |\langle I_z \rangle|)$  we take an average of the two extremes, as derived in the appendix. Integrating Eq. (3) over the survival distribution, characterized by the tunneling time  $\tau_{\text{out}}$ , finally yields the flip-flop probability

$$p_{\text{ff}} = \int_{t'=0}^{\infty} dt' \frac{e^{-t'/\tau_{\text{out}}}}{\tau_{\text{out}}} p_{|M+1, \downarrow\rangle} = \frac{2\gamma\tau_{\text{out}}^2}{(4\gamma + \xi)\tau_{\text{out}}^2 + \hbar^2}.$$

Referring to previous work on dynamical nuclear polarization, the result is of a rather standard form, with  $\tau_{\text{out}}$  as correlation time [5, 6]. Since we operate at rather low magnetic fields, where the “bright”  $|\uparrow\downarrow\rangle, |\downarrow\uparrow\rangle$   $X^0$  states are split from the “dark”  $|\uparrow\uparrow\rangle, |\downarrow\downarrow\rangle$   $X^0$  states by far more than a hundred  $\mu\text{eV}$  [2, 7], spin flip-flops among electron and nuclei are negligible in the presence of a hole.

### III. NUCLEAR SPIN DYNAMICS AND STABLE SOLUTIONS

The combination of the electron spin creation rate and the flip-flop probability results in a dynamic equation for the nuclear spin polarization  $\langle I_z \rangle$ . It is driven up depending on  $p_{|\uparrow\downarrow\uparrow\rangle}$ , down depending on  $p_{|\downarrow\uparrow\downarrow\rangle}$ , and decays in the absence of driving with rate  $\Gamma_{\text{leak}}$ . With  $\tau_1 (\sim \text{ns}) \gg \tau_{\text{out}} (\sim \text{ps})$ , the cycle round-trip time is simply  $\tau_1$  and the dynamic equation reads

$$\frac{d}{dt} \langle I_z \rangle \simeq \frac{p_{\text{ff}}}{N\tau_1} [p_{|\uparrow\downarrow\uparrow\rangle} - p_{|\downarrow\uparrow\downarrow\rangle}]_t = \tau_1 - \Gamma_{\text{leak}} \langle I_z \rangle. \quad (4)$$

The flip-flop probability  $p_{\text{ff}}$  is a function of  $\langle I_z \rangle$ , the populations  $p_{|\uparrow\downarrow\uparrow\rangle}, p_{|\downarrow\uparrow\downarrow\rangle}$  are functions of both nuclear spin polarization and laser detuning. We solve Eq. (4) numerically to find stable values of  $\langle I_z \rangle$  as a function of detuning  $\hbar\delta$ . Figure 2 plots the dynamic equation (4) as a function of nuclear spin polarization, parameters as in section V, as the laser is tuned through the bistability. Stable nuclear spin polarizations are found where  $\frac{d}{dt} \langle I_z \rangle$  crosses zero with negative slope. The stable nuclear spin polarizations are directly related to the Overhauser shift  $\Delta_n$  observed in the experiment. Comparing the  $X^{1-}$  emission energies  $E(\sigma^{+/-})$  measured for  $\sigma^{+/-}$  polarization,

$$E(\sigma^+) - E(\sigma^-) = g_X \mu_B B_z + \Delta_n \equiv g_X^{\text{eff}} \mu_B B_z,$$

where we take  $\Delta_n = -A \langle I_z \rangle$  according to Eq. (1). Figure 1 (right) shows four counts-energy spectra measured in the region of bistability and fitted to Lorentzian curves, where  $E(\sigma^{+/-})$  are given by the centers of the respective fit functions. It illustrates a key feature of the presented scheme, the tuning of resonance energies via control over the net polarization in the nuclear spin bath. In [1], a change from  $-45 \mu\text{eV}$  to  $+20 \mu\text{eV}$  in the total electron Zeeman splitting  $g_e^{\text{eff}} \mu_B B_z = g_e \mu_B B_z + A \langle I_z \rangle$  is observed, so that the sign of the effective electron g-factor  $g_e^{\text{eff}}$  can be *inverted* and, using the continuous change in  $\langle I_z \rangle$  at more

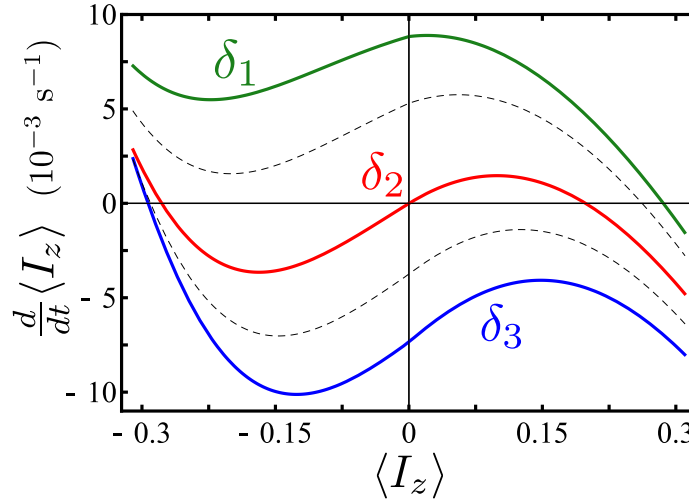

FIG. 2. Simulation of  $\frac{d}{dt}\langle I_z \rangle$ , Eq. (4), with the parameters as summarized in section V and  $B_z = +0.5$  T. Stable nuclear spin polarizations are found where the horizontal axis is crossed with negative slope. For  $\hbar\delta_1 = -42$   $\mu\text{eV}$  (green), one solution exists at positive  $\langle I_z \rangle$ . For  $\hbar\delta_2 = -38.5$   $\mu\text{eV}$  (red), an additional stable solution exists at negative nuclear spin polarization, leading to a bistability. The solution at positive  $\langle I_z \rangle$  disappears when the laser detuning is further increased,  $\hbar\delta_3 = -36$   $\mu\text{eV}$  (blue). The theoretical width of the bistable region is 2  $\mu\text{eV}$ , and in general depends on the various input parameters. Widths  $> 10$   $\mu\text{eV}$  are achievable.

positive laser energies, tuned precisely to zero. Accordingly, the effective exciton g-factor  $g_X^{\text{eff}}$  is tuned from 2.6 to 0.3, and tuning  $g_X^{\text{eff}}$  through zero should easily be possible with an optimized cycle.

The Lorentzians fitted to the experimental data not only yield the line energies (center), but also the line intensities (area under the curve), denoted as  $S(\sigma^{+/-})$ . In terms of the theoretical model, the  $\sigma^+$  ( $\sigma^-$ ) intensity corresponds to the rate of creating an  $\uparrow$  ( $\downarrow$ ) electron via  $X^{1-}$  recombination. For each stable solution of  $\frac{d}{dt}\langle I_z \rangle = 0$  we can hence calculate the  $\sigma^{+/-}$  emission intensity and the associated degree of polarization,

$$P \equiv \frac{S(\sigma^+) - S(\sigma^-)}{S(\sigma^+) + S(\sigma^-)} = \frac{p_{|\uparrow\downarrow\uparrow\rangle} - p_{|\downarrow\uparrow\downarrow\rangle}}{p_{|\uparrow\downarrow\uparrow\rangle} + p_{|\downarrow\uparrow\downarrow\rangle}} \Big|_{t=\tau_1}.$$

#### IV. CALCULATION OF NUCLEAR SPIN DISTRIBUTION WIDTH

The model also provides insight into the width of the nuclear spin distribution. The typical fluctuating nuclear magnetic field seen by the electron spin via the hyperfine interaction is  $\sim A/(g_e\mu_B\sqrt{N})$  [8, 9]. This corresponds to a fluctuation of the nuclear spin polarization  $\langle I_z \rangle$  by typically  $1/\sqrt{N}$  and, in terms of the associated Gaussian distribution function, a variance of  $\sigma^2 \sim 1/N$ . To calculate the nuclear spin distribution in the presence of the laser field, we follow the steps as summarized in Ref. [10] (supplementary information). Starting from a basic rate equation, reformulation in the continuum limit results in a Fokker-Planck equation which is solved for stable nuclear spin distributions. These solutions are of the form  $e^{F(\langle I_z \rangle)}$ ; expanding the argument  $F$  to second order in  $\langle I_z \rangle$  around the stable nuclear spin polarization  $I_{z,0}$  yields the variance of the distribution. One finds

$$\sigma^2 = \frac{1}{2N} \frac{\Gamma_t}{\frac{\partial}{\partial \langle I_z \rangle} \left( -\frac{d}{dt} \langle I_z \rangle \right)} \Big|_{\langle I_z \rangle = I_{z,0}},$$

where  $\Gamma_t$  is the total spin flip rate divided by  $N$ ,

$$\Gamma_t = \frac{p_{\text{ff}}}{N\tau_1} [p_{|\uparrow\downarrow\uparrow\rangle} + p_{|\downarrow\uparrow\downarrow\rangle}]_{t=\tau_1} + \Gamma_{\text{leak}}|\langle I_z \rangle| + 2\Gamma_{\text{leak}}.$$

The additional  $2\Gamma_{\text{leak}}$  accounts for intrinsic diffusion and ensures that  $\sigma^2 = 1/N$  in the absence of a laser field. The simulation shows that the cycle in the particular experiment in [1] results in a reduction of the variance by a small factor ( $\sim 1.7$ ). However, the scheme is capable of narrowing the variance of the nuclear spin distribution by factors  $\sim 5$  (similar to the numbers reported e.g. in [11]) by increasing the tunneling times slightly.

## V. INPUT PARAMETERS

The parameters for the simulation are set by in situ characterization of the quantum dot, comparison with previous experiments on the same sample, and by making small tweaks to fit the experimental data presented in Fig. 2 of [1]. The main features – an abrupt inversion in the polarization of both photoluminescence (PL) and nuclear spins, followed by continuous tuning through zero – are not sensitive to the parameters in the calculation. Reproducing the exact experimental results is however sensitive to the exact parameters, in particular  $\hbar\omega_{fs}$ ,  $\tau_{in}$ ,  $\tau_{out}$ , and  $\Gamma_{leak}$ .

- The Rabi energy  $\hbar\Omega$  is proportional to the oscillating electric field and can therefore be estimated from the power density at the quantum dot. This gives us a rough estimate of  $\hbar\Omega$ . A more precise determination is taken from [12] in which the Rabi energy is measured directly from the Autler-Townes splitting in a pump-probe experiment. This experiment used the same microscope and a sample from the same wafer as the present experiment. Given a laser power of 13 kW/cm<sup>2</sup> and the values reported in [12], we determine  $\hbar\Omega = 23 \mu\text{eV}$ .
- The fine structure splitting  $\hbar\omega_{fs}$  is highly scattered from dot to dot in this sample [13], 40  $\mu\text{eV}$  is taken here, largely by fitting the results of the model to the experimental data.
- For the exciton recombination times  $\tau_0$  ( $X^0$ ) and  $\tau_1$  ( $X^{1-}$ ), we take  $\tau_0 = 0.75$  ns and  $\tau_1 = 0.95$  ns from lifetime measurements of quantum dots in this wafer [14]. There is a systematic increase in the recombination lifetimes on going from  $X^0$  to  $X^{1-}$ , and a systematic dependence on the  $X^0$  exciton energy. Both these factors are included.
- The time  $\tau_{in} = 35$  ps for tunneling *into* the dot is estimated from  $\tau_0$  and the ratio of  $X^0$ ,  $X^{1-}$  PL intensities in the hybridization region. The tunneling time for tunneling *out* of the dot is smaller as the electron is now above rather than below the Fermi energy (where the energy barrier is thinner). Experiments probing the spin cotunneling rate [15] and the photoluminescence in the hybridization region [16] on dots similar to the one used here point to a  $\tau_{out}$  time of  $\sim 10$  ps. Fine tuning by fitting the experimental data gives  $\tau_{out} = 5$  ps.
- $N$ , the number of quantum dot nuclear spins, is estimated from the extent of the electron wave function. The ground state for harmonic confinement,

$$\psi_1(\vec{r}) = C_1 e^{-\frac{1}{2} \left( \frac{x^2}{l_x^2} + \frac{y^2}{l_y^2} + \frac{z^2}{l_z^2} \right)},$$

is replaced by a step function  $\psi_2$  of amplitude  $C_2 = C_1/\sqrt{e}$ , the value where  $|\psi_1|^2 4\pi r^2 dr$ , with  $r = \sqrt{x^2 + y^2 + z^2}$ , peaks in the simple case of spherical symmetry. The lengths  $l_i$  are related to the quantization energies  $\hbar\omega_i$  and effective electron mass  $m^*$  via  $l_i = \sqrt{\hbar/(m^*\omega_i)}$ . With  $\hbar\omega_{x,y} = 30$  meV [17] and  $\hbar\omega_z = 95$  meV [18] we calculate  $N = 8.5 \times 10^4$  as the number of nuclear spins covered by  $\psi_2$ . This result is consistent with a measurement of the fluctuations in the Overhauser field [19] (see Section IV).

- The electron g-factor is  $g_e = -0.5$  as determined by optically detected single electron spin resonance performed on a dot in a very similar sample to the one used here [19]. For the exciton,  $g_X = 1.55$  was measured by assuming that at large detunings, where  $E(\sigma^+) - E(\sigma^-)$  takes on a constant value,  $\Delta_n$  changes sign but not magnitude on switching the pump polarization,

$$g_X \simeq \frac{1}{2\mu_B B_z} \left( [E(\sigma^+) - E(\sigma^-)]_{\sigma^+ \text{ pump}} + [E(\sigma^+) - E(\sigma^-)]_{\sigma^- \text{ pump}} \right).$$

- The order of magnitude of the spin depolarization rate  $\Gamma_{leak}$  results from direct experimental observations. As demonstrated in [1], the system always preserves its state when the laser, tuned to the region of bistability, is turned off and back on after times  $\sim 30$  s. For times  $> 1$  min this is no longer true, pointing towards leakage rates of  $\sim 0.01$  to  $0.1 \text{ s}^{-1}$ . This measures the decay of the nuclear spin polarization with the dot in the vacuum state,  $|0\rangle$ . Optical pumping in the hybridization region causes the dot, averaged over time, to be partially occupied such that the relevant value of  $\Gamma_{leak}$  is likely to be larger. We take  $\Gamma_{leak} = 0.1 \text{ s}^{-1}$  here as it gives the best fit to the experimental data.

### Appendix: Flip-flop term in an effective 2D system

Since  $\langle I_z \rangle$  is observed via the Overhauser shift  $\Delta_n = -A\langle I_z \rangle$ , we calculate the flip-flop probability as a function of nuclear spin polarization. Letting the total nuclear spin  $\vec{z}$  projection, in units of  $\hbar$ , be  $M$ ,

$$M = \sum_k I_k^z = N\langle I_z \rangle,$$

then the state of the nuclear spin bath is a linear superposition of states  $|J, M, \lambda_M^J\rangle$ , where  $M$  is fixed,  $|M| \leq J \leq NI$  is the quantum number for the total spin length, and  $\lambda_M^J$  is an additional quantum number whose range depends on  $M$  and  $J$ , such that

$$\sum_{J=0(\frac{1}{2})}^{NI} \sum_{M'=-J}^J \sum_{\lambda} |J, M', \lambda_{M'}^J\rangle \langle J, M', \lambda_{M'}^J| = \mathbb{1}.$$

Assuming the free electron has spin up, the Hamiltonian  $\hat{H}_{\text{ext}} + \hat{H}_{\text{hf}}$  given in Eq. (2) couples the states  $|J, M, \lambda_M^J, \uparrow\rangle$  with states  $|J, M+1, \lambda_{M+1}^J, \downarrow\rangle$ , where the electron spin was simply added to the notation. For given  $M$ , considering the number of  $\sim 10^5$  nuclear spins, the system of interest is therefore high dimensional. However, it can be reduced to an effective 2D system.

Since the energy depends only on the electron spin and the total nuclear spin  $\vec{z}$  polarization, all states associated with  $|\uparrow\rangle, |\downarrow\rangle$  have the same eigenenergy  $E_1, E_2$  respectively. The population at time  $t' = 0$  is distributed among the states  $|J, M, \lambda_M^J, \uparrow\rangle$ , which we formally replace by a state  $|M, \uparrow\rangle$  with 100% occupation probability and eigenenergy  $E_1$ . This state  $|M, \uparrow\rangle$  is coupled to the states with nuclear spin  $\vec{z}$  projection  $(M+1)$  via the flip-flop term in the contact hyperfine Hamiltonian, Eqs. (1, 2). For the estimate of the spin flip probability, it only matters whether the system occupies state  $|M, \uparrow\rangle$  or any of the other states  $|J, M+1, \lambda_{M+1}^J, \downarrow\rangle$ . Therefore the dynamics can equivalently be calculated in a reduced system, where the  $|J, M+1, \lambda_{M+1}^J, \downarrow\rangle$  are replaced by the effective state  $|M+1, \downarrow\rangle$  of eigenenergy  $E_2$  and effective coupling  $\gamma$  where

$$\gamma \equiv \left| \langle M+1, \downarrow | \hat{H}_{\text{hf}} | M, \uparrow \rangle \right|^2 = \sum_{J=|M+1|}^{NI} \sum_{\lambda} \left| \langle J, M+1, \lambda_{M+1}^J, \downarrow | \hat{H}_{\text{hf}} | M, \uparrow \rangle \right|^2. \quad (\text{A.1})$$

The value of  $\gamma$  strongly depends on the system. In the following, the two extremes of a strongly correlated and a fully uncorrelated system will be considered.

#### Strong correlation

As a first limit, we assume a highly coherent system free of further interactions, such that transitions  $J \leftrightarrow J+1$  are impossible. The relevant flip-flop term in the hyperfine Hamiltonian is

$$\frac{A}{2N} \sum_k I_k^+ S^- = \frac{A}{2N} J^+ S^-,$$

where  $J^+ \equiv \sum_k I_k^+$  acts as a raising operator for the total spin. Its effect on a state  $|J, M, \uparrow\rangle$  ( $\lambda$  irrelevant) within  $|M, \uparrow\rangle$  is

$$\frac{A}{2N} J^+ S^- |J, M, \uparrow\rangle = \frac{A}{2N} \sqrt{(J-M)(J+M+1)} |J, M+1, \downarrow\rangle, \quad (\text{A.2})$$

which breaks down as soon as the expression under the square root is zero. Starting from an unpolarized system, the typical order of magnitude for the starting value of  $J$  can be estimated from the infinite temperature limit:

$$\begin{aligned} \bar{J}(\bar{J}+1) &= \langle \vec{J} \cdot \vec{J} \rangle = \sum_{k \neq k'} \langle \vec{I}_k \cdot \vec{I}_{k'} \rangle + \sum_k \langle \vec{I}_k \cdot \vec{I}_k \rangle = \sum_k \langle \vec{I}_k \cdot \vec{I}_k \rangle = NI(I+1), \\ \bar{J} &\simeq \sqrt{N} \sqrt{I(I+1)}. \end{aligned}$$

Given this value, Eq. (A.2) typically approaches zero when  $|\langle I_z \rangle| \simeq \sqrt{I(I+1)/N}$ . For  $N = 8.5 \times 10^4$  and  $I = 2.25$ , these so-called “dark” states would therefore be reached at nuclear spin polarizations of less than 1% in both positive and negative  $\vec{z}$  directions. This is in clear contradiction with the experiment, where polarizations of  $\sim 20\%$  were measured and dark states were not observed.

No correlation

In the other extreme, we take an uncorrelated system without transverse spin coherence, so that there is no correlation among the  $x, y$  components of the nuclear spins. Starting from Eq. (A.1),

$$\begin{aligned}
 \gamma &= \sum_{J=|M+1|}^{NI} \sum_{\lambda} \left| \langle J, M+1, \lambda_{M+1}^J | \hat{H}_{\text{hf}} | M, \uparrow \rangle \right|^2 = \frac{A^2}{4N^2} \sum_{J=|M+1|}^{NI} \sum_{\lambda} \left| \langle J, M+1, \lambda_{M+1}^J | \sum_k I_k^+ | M \rangle \right|^2 \\
 &= \frac{A^2}{4N^2} \sum_{k, k'} \langle M | I_k^- \underbrace{\sum_{J=|M+1|}^{NI} \sum_{\lambda} |J, M+1, \lambda_{M+1}^J\rangle \langle J, M+1, \lambda_{M+1}^J|}_{\text{equivalent to } \mathbb{1}, \text{ only non-zero contribution}} I_{k'}^+ | M \rangle \\
 &= \frac{A^2}{4N^2} \underbrace{\sum_{k \neq k'} \langle M | I_k^- I_{k'}^+ | M \rangle}_{=0} + \frac{A^2}{4N^2} \sum_k \langle M | I_k^- I_k^+ | M \rangle \\
 &= \frac{A^2}{4N^2} \sum_k \langle M | (I^2 + I - (I_k^z)^2 - I_k^z) | M \rangle \simeq \frac{A^2}{4N} (I^2 + I - \langle I_z \rangle^2 - \langle I_z \rangle).
 \end{aligned}$$

This calculation represents the nuclear spin system when coherence in the nuclear spin bath is lost between two cycles via various mechanisms such as the dipole-dipole interaction among the nuclear spins. However, these interactions are weak and the cycle round-trip time is very short,  $\sim 1$  ns, so that this limit isn't realistic either.

Considering  $I = 2.25$ , we therefore take  $\gamma = \frac{A^2}{4N} (I - |\langle I_z \rangle|)$  as a compromise of the two extremes. An analogous calculation can be carried out when the electron spin is initially down. It is clear that  $\gamma$  must decrease as  $|\langle I_z \rangle|$  increases. The exact functional form of  $\gamma$  is not crucial to describe theoretically the main experimental phenomena but it is important to describe the experimental results quantitatively.

- 
- [1] C. Kloeffer, P. A. Dalgarno, B. Urbaszek, B. D. Gerardot, D. Brunner, P. M. Petroff, D. Loss, and R. J. Warburton, Phys. Rev. Lett. **106**, 046802 (2011).
  - [2] M. Bayer, G. Ortner, O. Stern, A. Kuther, A. A. Gorbunov, A. Forchel, P. Hawrylak, S. Fafard, K. Hinzer, T. L. Reinecke, S. N. Walck, J. P. Reithmaier, F. Klopfer and F. Schäfer, Phys. Rev. B **65**, 195315 (2002).
  - [3] H. P. Breuer and F. Petruccione, *The Theory of Open Quantum Systems* (Oxford University Press, Oxford, 2002), Chapter 3.
  - [4] W. A. Coish and J. Baugh, Phys. Status Solidi B **246**, 2203 (2009).
  - [5] B. Eble, O. Krebs, A. Lemaître, K. Kowalik, A. Kudelski, P. Voisin, B. Urbaszek, X. Marie, and T. Amand, Phys. Rev. B **74**, 081306(R) (2006).
  - [6] A. Abragam, *Principles of Nuclear Magnetism* (Oxford University Press, Oxford, 1961), Chapter 8.
  - [7] F. Klotz, V. Jovanov, J. Kierig, E. C. Clark, M. Bichler, G. Abstreiter, M. S. Brandt, J. J. Finley, H. Schwager, and G. Giedke, Phys. Rev. B **82**, 121307(R) (2010).
  - [8] A. V. Khaetskii, D. Loss, and L. Glazman, Phys. Rev. Lett. **88**, 186802 (2002).
  - [9] M. I. Dyakonov and V. I. Perel, in *Optical Orientation* (North-Holland, Amsterdam, 1984), p. 11.
  - [10] I. T. Vink, K. C. Nowack, F. H. L. Koppens, J. Danon, Y. V. Nazarov, and L. M. K. Vandersypen, Nature Phys. **5**, 764 (2009).
  - [11] C. Latta, A. Högele, Y. Zhao, A. N. Vamivakas, P. Maletinsky, M. Kroner, J. Dreiser, I. Carusotto, A. Badolato, D. Schuh, W. Wegscheider, M. Atatüre, and A. Imamoglu, Nature Phys. **5**, 758 (2009).
  - [12] B. D. Gerardot, D. Brunner, P. A. Dalgarno, K. Karrai, A. Badolato, P. M. Petroff, and R. J. Warburton, New J. Phys. **11**, 013028 (2009).
  - [13] S. Seidl, B. D. Gerardot, P. A. Dalgarno, K. Kowalik, A. W. Holleitner, P. M. Petroff, K. Karrai, and R. J. Warburton, Physica E **40**, 2153 (2008).
  - [14] P. A. Dalgarno, J. M. Smith, J. McFarlane, B. D. Gerardot, K. Karrai, A. Badolato, P. M. Petroff, and R. J. Warburton, Phys. Rev. B **77**, 245311 (2008).
  - [15] J. M. Smith, P. A. Dalgarno, R. J. Warburton, A. O. Govorov, K. Karrai, B. D. Gerardot, and P. M. Petroff, Phys. Rev. Lett. **94**, 197402 (2005).
  - [16] P. A. Dalgarno, M. Ediger, B. D. Gerardot, J. M. Smith, S. Seidl, M. Kroner, K. Karrai, P. M. Petroff, A. O. Govorov, and R. J. Warburton, Phys. Rev. Lett. **100**, 176801 (2008).
  - [17] C. Schulhauser, D. Haft, R. J. Warburton, K. Karrai, A. O. Govorov, A. V. Kalameitsev, A. Chaplik, W. Schoenfeld, J. M. Garcia, and P. M. Petroff, Phys. Rev. B **66**, 193303 (2002).
  - [18] R. J. Warburton, C. Schulhauser, D. Haft, C. Schäflein, K. Karrai, J. M. Garcia, W. Schoenfeld, and P. M. Petroff, Phys. Rev. B **65**, 113303 (2002).
  - [19] M. Kroner, K. M. Weiss, B. Biedermann, S. Seidl, S. Manus, A. W. Holleitner, A. Badolato, P. M. Petroff, B. D. Gerardot, R. J. Warburton, and K. Karrai, Phys. Rev. Lett. **100**, 156803 (2008).
